# Supplementary material for: Distributionally Robust Lyapunov Function Search Under Uncertainty
Source: arXiv:2212.01554 source file (2024-07-11)
Supplement: Supplementary file 1 [file Appendix_DRCLF_SOS.tex]

\section{SOS Formulation for DR-CLF}
We use $\tilde{f}(\bfx)$ and $\tilde{g}(\bfx)$ to denote terms in the nominal dynamics. A CLF QP subject to the nominal dynamics is given as follows:
\begin{equation}
\begin{aligned}
\label{eq: clf_qp_nomi}
    &\min_{\bfu \in \calU} \| \bfu\|^2,  \\
    \mathrm{s.t.} \, \, &L_{\tilde{f}} V(\bfx) + L_{\tilde{g}} V(\bfx)\bfu + \alpha_V (V(\bfx)) \leq 0.
\end{aligned}
\end{equation}
Assume $V$ is a valid CLF and  $L_{\tilde{g}} V(\bfx) = \mathbf{0}$ only if $L_{\tilde{f}} V(\bfx) + \alpha_V (V(\bfx)) < 0$. The closed-form solution to \eqref{eq: clf_qp_nomi} is given by:
\begin{equation} 
\label{sol: nomi_u}
	\tilde{\bfu} = \begin{cases}
	    -L_{\tilde{g}} V(\bfx)^{\top} \frac{L_{\tilde{f}} V(\bfx) + \alpha_V (V(\bfx))}{\| L_{\tilde{g}} V(\bfx) \|^2}, & L_{\tilde{f}} V(\bfx) + \alpha_V (V(\bfx)) > 0, \\
		\mathbf{0}, & L_{\tilde{f}} V(\bfx) + \alpha_V (V(\bfx)) \leq 0.
		\end{cases}\\
\end{equation}
First, we need to make sure that the CLF QP subject to nominal system dynamics is feasible. Let $l_1, l_2$ be positive definite, SOS polynomials, we need to ensure: 
\begin{align}
\label{cond: nomi_qp_feas}
    & V(\bfx) = \sum_{i=1}^{d} c_i \bfx^i, \ c_0 = 0, \notag \\
    & \left\{ \bfx \in \calX | V(\bfx) \leq 0, l_1(\bfx) \neq 0 \right\} = \emptyset, \notag \\
    & \left\{\bfx \in \calX | L_{\tilde{g}} V(\bfx) = \mathbf{0}, L_{\tilde{f}} V(\bfx) + \alpha_V (V(\bfx)) \geq 0, l_2(\bfx) \neq 0 \right\} = \emptyset.
\end{align}
Also, we want our CLF $V$ to be distribuionally robust subject to the nominal controller given by \eqref{sol: nomi_u}. To achieve this, we need to satisfy \eqref{eq: drccp_clf_constraint} with $\beta(\bfx) = [1, \tilde{\bfu}^{\top}]^{\top}$. Noting that for $L_{\tilde{f}} V(\bfx) + \alpha_V (V(\bfx)) \geq 0$, we have $\beta(\bfx)^{\top}q(\bfx) + a V(\bfx) = 0$, so in this case, we only need to ensure the following set is empty:
\begin{equation}
\label{cond: dr_nz_u}
    \left\{ \bfx \in \calX | L_{\tilde{f}} V(\bfx) + \alpha_V (V(\bfx)) \geq 0, \alpha [1, \tilde{\bfu}^{\top}]\bfR(\bfx)\bfxi_i \pm r  [1, \tilde{\bfu}^{\top}]\bfR(\bfx)_j \geq 0, l_3(\bfx) \neq 0  \right\}
\end{equation}
for all $i = 1,2 \dots, N, \quad \forall j = 1,2 \dots, k$. Where $l_3$ be a positive definite, SOS polynomial.

For the case $L_{\tilde{f}} V(\bfx) + \alpha_V (V(\bfx)) \leq 0$, we simply replace $\beta(\bfx) = [1, \tilde{\bfu}^{\top}]^{\top}$ with $\beta(\bfx) = [1, \mathbf{0}_m^{\top}]^{\top}$, and make sure the following set is empty:
\begin{equation}
\label{cond: dr_z_u}
    \left\{ \bfx \in \calX | -L_{\tilde{f}} V(\bfx) - \alpha_V (V(\bfx)) \geq 0, \alpha  \dot{V}(\bfx, \bfxi_i) \pm r  [1, \mathbf{0}_m^{\top}]\bfR(\bfx)_j \geq 0, l_4(\bfx) \neq 0  \right\}
\end{equation}
for all $i = 1,2 \dots, N, \quad \forall j = 1,2 \dots, k$. Where $l_4$ be a positive definite, SOS polynomial.
To ease notation, we set $\tilde{F}_V(\bfx) = L_{\tilde{f}} V(\bfx) + \alpha_V (V(\bfx))$. Applying P-satz to \eqref{cond: nomi_qp_feas}, we have the following SOS constraint \cite{TanSearchingFC}:
\begin{align}
\label{cond: nomi_qp_feas_sos}
    & V(\bfx) = \sum_{i=1}^{d} c_i \bfx^i, \ c_0 = 0; \; \; V(\bfx) - \epsilon\|\bfx\|_2^2 \in \text{SOS}(\bfx); \notag \\
    & -s_1\tilde{F}_V(\bfx) - L_{\tilde{g}} V(\bfx) \bfp_1 - l_2 
    \in \text{SOS}(\bfx),
\end{align}
where $\bfp_1$ is a vector of dimension $m$ with each element a polynomial of two variables and $s_1 \in \text{SOS}$. Similarly, we reformulate \eqref{cond: dr_nz_u} and \eqref{cond: dr_z_u} as the following SOS constraints:

%\TODO{Problem: $[1, \tilde{\bfu}^{\top}]^{\top}$ is a function of $V$ and $\bfR(\bfx)$ is a function of $V$ as well, causing non-linearity in decision variables.}
%\left\{ \bfx \in \calX | -L_{\tilde{f}} V(\bfx) - \alpha_V (V(\bfx)) \geq 0, \alpha  [1, \mathbf{0}_m^{\top}]\bfR(\bfx)\bfxi_i + \alpha (L_{\tilde{f}} V(\bfx) + \alpha_V (V(\bfx))) \pm r  [1, \mathbf{0}_m^{\top}]\bfR(\bfx)_j \geq 0, l_4(\bfx) \neq 0  \right\}
