# Supplementary material for: Distributionally Robust Lyapunov Function Search Under Uncertainty
Source: arXiv:2212.01554 source file (2024-07-11)
Supplement: Supplementary file 2 [file Appendix_Yi.tex]

\section{Miscellaneous Things}
\label{sec: quantitative_results}

\begin{table}[htb]
	\centering
	\caption{9 Training Samples. The results are shown in the following format: $a\% \mid b\%$, where $a\%$ denotes the violation rate of each formulation: (validations with $\dot{V} > 0$)/(total validations), and $b\%$ denotes the average violation area over all simulations: (data points with $\dot{V} > 0$)/(total data points).
    For each case, 5000 realizations of the online true uncertainty $\bfxi^*$ have been sampled from a uniform distribution with $\bfxi^*_1 \in \calU_{[1,4]}, \bfxi^*_2 \in \calU_{[1,2]}$ and a Gaussian distribution with $\bfxi^*_1 \in \calN(4,1.5), \bfxi^*_2 \in \calN(1,1.5)$ for Case 1, and a uniform distribution with $\bfxi^*_1 \in \calU_{[5,7]}, \bfxi^*_2 \in \calU_{[-1,1]}$ and a Gaussian distribution with $\bfxi^*_1 \in \calN(7,1), \bfxi^*_2 \in \calN(1,1)$ for Case 2. 
    For each realization, the learned Lyapunov function has been tested on 10000 data points generated in the same region: $x_1, x_2 \in [-2,2]$. If $\dot{V} > 0$ at any of those data points, then the realization is considered to be a violation.
    }
	\scalebox{1}{
    \begin{tabular}{ccccc}
		\toprule 
        Formulations & Case 1 Uniform & Case 1 Gaussian & Case 2 Uniform & Case 2 Gaussian \\
		\midrule  
		SOS & 14.28\% $\mid$ 0.94\% & 12.14\% $\mid$ 1.53\% & 100\% $\mid$ 15.52\% & 100\% $\mid$ 18.55\% \\
        CC-SOS & 11.78\% $\mid$ 0.89\% & 8.30\% $\mid$ 1.53\% & 0.00\% $\mid$ 0.00\% & 5.10\% $\mid$ 0.04\% \\
        DRCC-SOS & 0.02\% $\mid$ 0.00\% & 5.24\% $\mid$ 0.80\% & 0.00\% $\mid$ 0.00\% & 1.64\% $\mid$ 0.01\% \\
		NN & 16.74\% $\mid$ 0.78\% & 10.24\% $\mid$ 0.96\% & 100\% $\mid$ 17.26\% & 100\% $\mid$ 18.55\% \\
        CC-NN & 9.56\% $\mid$ 0.09\% & 0.82\% $\mid$ 0.10\% & 0.00\% $\mid$ 0.00\% & 5.10\% $\mid$ 0.0376\% \\
        DRCC-NN & 4.32\% $\mid$ 0.02\% & 3.58\% $\mid$ 0.02\% & 0.00\% $\mid$ 0.00\% & 1.64\% $\mid$ 0.01\% \\
		\bottomrule
	\end{tabular}}
\end{table}
For both cases, the CC-SOS and DRCC-SOS formulations outperform the conventional SOS formulation (no uncertainty considered). Also, the DRCC-SOS formulation outperforms the CC-SOS formulation for $\bfxi^*$ sampled from both uniform and Gaussian distributions (low violation rate and mean violation area). However, the improvement of the DRCC-SOS formulation over the CC-SOS formulation is not as significant as the improvement of the CC-SOS formulation over the SOS formulation, since the CC-SOS formulation is already conservative enough, the extra conservativeness DRCC-SOS introduces depends on the Wasserstein radius $r$, which cannot be chosen arbitrarily large otherwise the problem will be infeasible.
