# Supplementary material for: Distributionally Robust Lyapunov Function Search Under Uncertainty
Source: arXiv:2212.01554 source file (2024-07-11)
Supplement: Supplementary file 4 [file Appendix_proof.tex]

\section{Proofs}
\label{sec: proof}

\subsection{Distributionally Robust Loss Function Design For Uncertain ODEs}
\label{sec: dr_nn_lf_proof}

\subsection{Distributionally Robust Quadratic Program Reformulation}
\label{sec: drccp_qp_proof}

\KL{Should we provide a proof here?}
